# Supplementary material for: Initiating and monitoring the evolution of single electrons within atom-defined structures
Source: arXiv:1709.10091 source file (2018-05-29)
Supplement: Supplementary file 1 [file Supplementary_Information.pdf]

# Supplementary Information:
# Initiating and monitoring the evolution of single electrons within atom-defined structures

Mohammad Rashidi[1,2,3*], Wyatt Vine[1*], Thomas Dienel[1,2*], Lucian Livadaru[3], Jacob Retallick[4], Taleana Huff[1,3], Konrad Walus[4], Robert A. Wolkow[1,2,3]

[1]Department of Physics, University of Alberta, Edmonton, AB, Canada, T6G 2R3

[2]Nanotechnology Initiative, Edmonton, AB, Canada, T6G 2M9

[3]Quantum Silicon, Edmonton, AB, Canada, T6G 2M9

[4]Department of Electrical and Computer Engineering, University of British Columbia, Vancouver, BC, Canada, V6T 1Z4

*Authors contributed equally

Correspondence to: rashidi@ualberta.net, wyattvine@gmail.com, thdienel@gmail.com

**Table of Contents:**

- Definition and discussion of error rate
- Data processing for repeated line scan experiments and assignment of digital charge configurations
- Height-dependent contrast in Δ*f* images
- Frequency to force conversion
- Additional experimental data
- References for Supporting Information

**Error Rate:** Throughout measurements restricted to the *read*-regime we occasionally observed negative charges occupying both dangling bonds in a pair, despite this being unlikely due to Coulombic repulsion. We define these line scans as errors. While it was typically several percent we have achieved error rates of <1% (Supporting Information, Fig. S2). We have identified several contributing factors. (*i*) The *read* and *write* regimes are sensitive to the tip height (Fig. 2 and SI Fig. S3). Accordingly, we find that small changes in tip height (*e.g.* noise of the tuning fork's amplitude) can occasionally result in unintentional manipulation of the charge state of dangling bonds beneath the tip while in the *read*-regime. This can result in an increase to the apparent occupation of the structure (*e.g.* Fig. 2). It can also reduce the success-rate of charge manipulation in the *write*-regime. (*ii*) Sharp tips were found to more clearly resolve the two charge states of each dangling bond, *i.e.*, better signal to noise ratio. This reduces the number of incorrect charge state assignments, which are performed in a digital fashion. Similarly, with H-terminated tips, which can be effectively identified via force distance spectroscopy [1], it was more difficult to discriminate the two charge states of each dangling bond.

**Data processing for repeated line scan experiments and assignment of digital charge configurations:** Minimal data processing was performed, and raw data was used whenever possible. All experiments with repeated line scans were performed in constant height mode. For experiments performed entirely in the *read* regime, forward and backward line scans, which are saved in separate files by the control software, were aligned manually by removing an equal number of pixels at the start of both scans and zipped

together (step 1, Fig. S1b). Measurements often exceeded 30 minutes, over which time the tip would inevitably drift towards or away from the surface due to piezo creep and thermal drift. To account for this, a linear drift was subtracted from all measurements with repeated line scans by fitting the average $\Delta f$ for each line scan over the course of an experiment (step 2, Fig. S1c). In experiments where $\Delta f$ drifted by more than 2 Hz the entire run was rejected.

The $\Delta f$ value measured over each dangling bond was extracted by independently fitting each dangling bond associated peak in the line scans (defined by a 30-pixel window centered on their position) with a Gaussian function (step 3, Fig. S1d). Supporting Figure S1e,f shows the extracted $\Delta f$ values for two dangling bonds. The bistable behavior of each dangling bond is clearly visible.

Binary numbers were assigned to the charge states by making a single cut in $\Delta f$ (Fig. S1e,f demonstrate cuts). Dangling bonds with $|\Delta f|$ greater than the cut were assigned a negative charge state, while those with $|\Delta f|$ smaller than the cut were assigned a neutral charge state (Fig. S1e,f). Two additional steps were used to create the histograms in Fig. S3 and S4. First, the smallest $|\Delta f|$ in the set of the $\Delta f$ extracted for all the dangling bonds in an experiment (corresponding to a fit of the background) was set to 0 (step 4). Thus, the normalized $\Delta f$ for all the dangling bonds would be positive. Second, each $\Delta f$ was normalized by setting the average $\Delta f$ for the two isolated dangling bonds to 1.0 (step 5). Because the isolated dangling bonds were always negatively charged, a normalized $\Delta f$ of 1.0 corresponds to the average $\Delta f$ for a negatively charged dangling bond. Similar to the process above a single common cut in $\Delta f$ was used to assign charge states to the normalized data (step 6).

**Height-dependent contrast in $\Delta f$ images**: To provide additional insight to the qualitative behaviour of the $\Delta f$ signal above each species we measured site-specific force curves. The results are presented as Figure 3a and in Supporting Figure S5 which shows $\Delta f(z)$ signals obtained while approaching the tip to the corresponding sites. For large tip-surface separations (height range>0 pm) all three species exhibit an identical frequency shift, *i.e.* the $\Delta f(z)$ curves coincide and there is no contrast. As the tip approaches (approx. -200 to 0 pm), attractive van der Waals forces are observed first on the hydrogen atoms. As a result, vacancies and neutral DBs have smaller $|\Delta f|$ compared to the surrounding H atoms and appear as bright protrusions in $\Delta f$ images taken in this height range. Negatively charged DBs appear dark (large $|\Delta f|$) due to electrostatic contributions.

For tip offsets closer to the surface than -200pm, the tip enters the repulsive regime over hydrogen atoms. Consequently, the $|\Delta f|$ obtained over the neutral dangling bond becomes greater than that of the hydrogen resulting in a darker appearance of the DBs. The final feature of interest is a sharp step (approx. -300 pm) in the approach curve on the neutral DB, which we attribute to the charging of the dangling bond beneath the tip and the dark appearance (large $|\Delta f|$). As the tip is being retracted the charge remains at the site under the tip and the corresponding DB appears darker than hydrogen or neutral DBs in $\Delta f$ images. All images and line profiles for the *write* and *read* scans are well within the same height regime and no contrast inversion exists.

**Frequency to force conversion:** To reliably separate the short range forces measured over dangling bonds and hydrogen we took reference measurements over dimer vacancies (Fig. S4). [2, 3] We

performed our measurements of Δ*f(z)* at the various sites in a series while keeping the instrument in constant height mode. Repeatedly taking Δ*f(z)* spectra over hydrogen atoms throughout the experiment allowed us to determine the residual thermal drift and piezo artefacts. Afterwards we shifted the spectra relative to one another and calculated the minimum residual sum squared error of the shifted spectra

$$\Sigma\ (\Delta f(z)_{shifted} - \Delta f(z)_{reference})^2\ .$$

By comparing the determined optimum offset for each hydrogen spectrum we revealed linear drift within each set of measurements, which subsequently allows us to correct the tip offsets.

We used the Sader-Jarvis method [4] and corrections proposed by Giessibl [5] to convert the Δ*f(z)* spectra to force curves (Fig. S5). We assumed a cantilever stiffness of 1800 N/m but note that others have reported large uncertainties in this value. The uncertainty in our reported short range forces correspond to the standard deviation between the data and their optimal fit and so a linear correction to the forces and their corresponding uncertainties would result if a different stiffness was assumed.

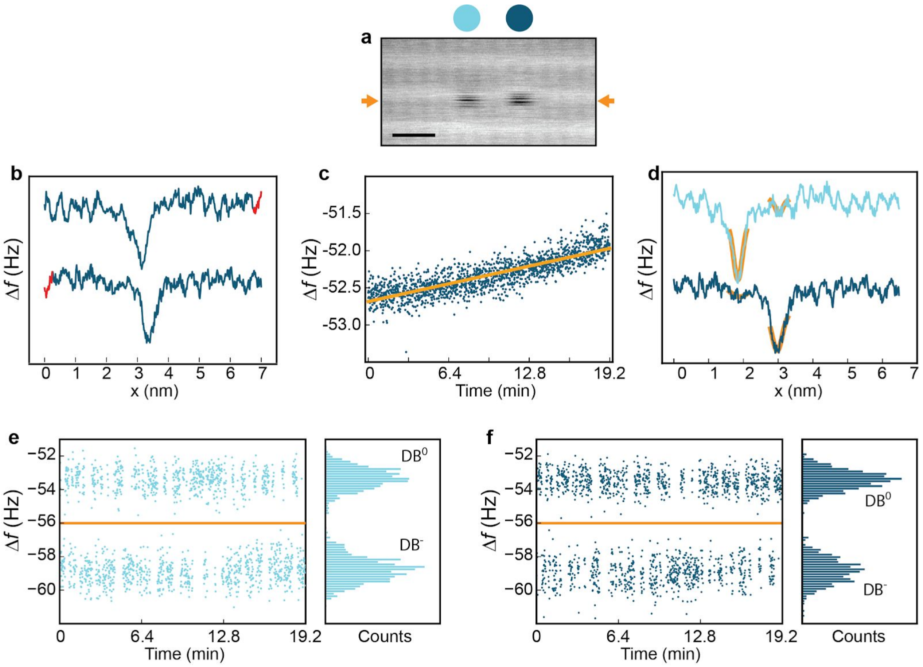


**Figure S1: Illustration of data processing routine for Δ*f* maps.** (**a**) Constant height Δ*f* image of a dangling bond structure taken at 0 V. The initial tip height is set on a hydrogen atom at -1.8 V and 50 pA before moving the tip 300 pm towards the surface. The scale bar is 1 nm. (**b**) Two sequential Δ*f* line scans demonstrate negative charge confined to the right-hand dangling bond (line scan width is larger than the window shown in (a), line scans are offset for clarity). The peaks are not aligned because they correspond to forward (top) and backward (bottom) line scans, which typically have a fixed offset due to piezo creep. The red tails on both line scans demonstrate the data that is chopped to align the scans. (**c**) The average Δ*f* of each line scan over the course of the entire experiment demonstrates that the tip was slowly drifting away from the sample. A linear fit of this data (orange line) is subtracted from the dataset. (**d**) Each line scan is fit with two gaussian peaks to extract the Δ*f* over each dangling bond (colour legend indicated above (a)). Note that for neutral dangling bonds this corresponds to a fit of the signal associated with hydrogen/noise. (**e-f**) The Δ*f* extracted for each dangling bond clearly displays two distinct states, which we assign to the negative and neutral charge states of each dangling bond. Each histogram has 75 equal width bins between Δ*f* = -62 and -51 Hz, and has an integrated area of 1.0.

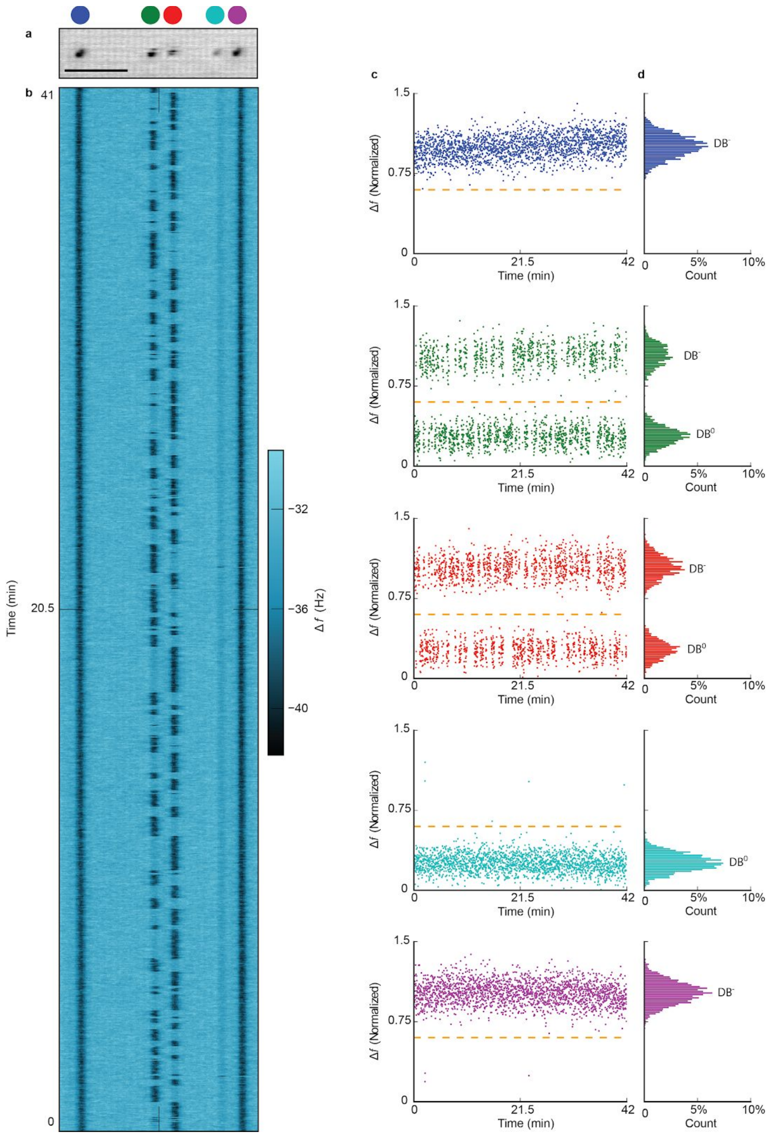


**Figure S2: Digitization of line scans of an asymmetric structure composed of five dangling bonds.** (**a**) Constant height Δ*f* image of the dangling bond structure at 0 V. (**b**) A line scan map composed of 2048 Δ*f* line scans acquired in the *read*-regime (-300 pm) over structure demonstrate. (**c**) The normalized Δ*f* acquired over each dangling bond throughout the course of the experiment demonstrates clearly that there are two charge states of each dangling bond (although only the green and red dangling bonds appear to fluctuate between them). With the normalizing procedure described above the negative dangling bond charge state is normalized to a Δ*f* of 1.0, and the Δ*f* of the neutral dangling bond state is centered approximately at 0.25. The orange dotted lines demonstrate that a single common cut of Δ*f* = 0.6 in the normalized data can be used to digitize the charge state of the structure with each line scan. (**d**) Histograms of the normalized Δ*f* for each dangling bond reveal that the Δ*f* corresponding to the two charge states of each dangling bond have a Gaussian distribution. Upon assigning binary numbers to this dataset it was found that in <1% of the line scans the charge configuration corresponded to having a third negative charge in the four paired dangling bonds. Each histogram has 75 equal width bins between Δ*f*(normalized) = 0 and 1.5, and has an integrated area of 1.0.

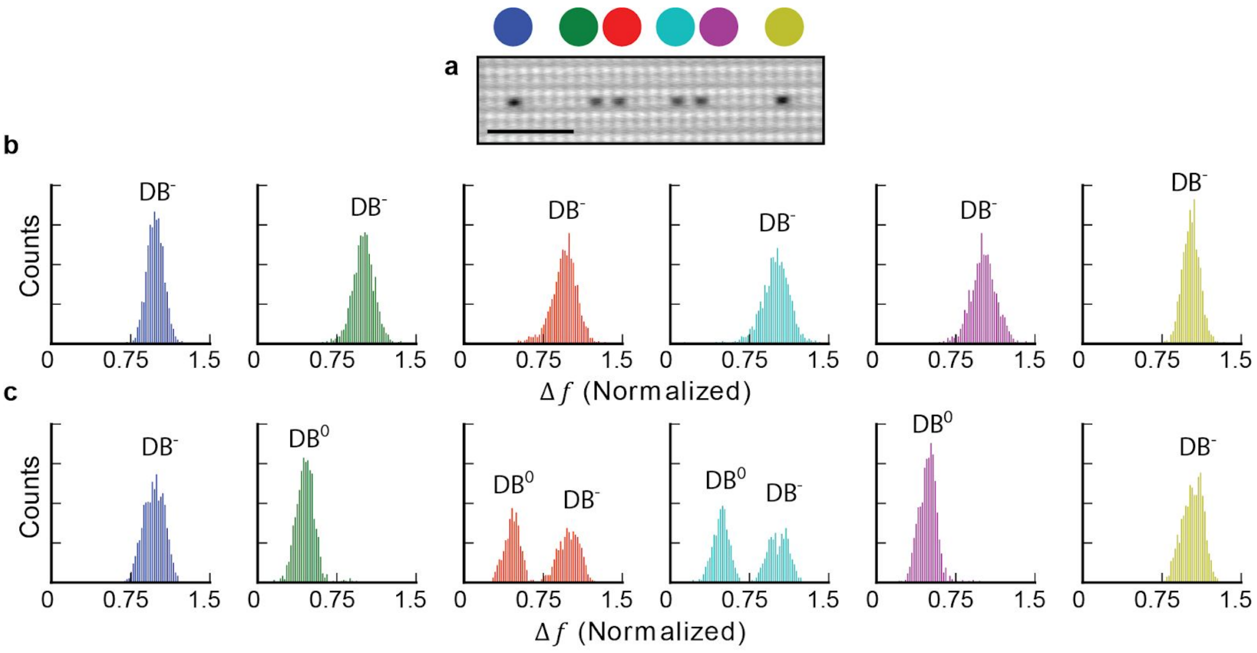


**Figure S3: Histograms of the normalized $\Delta f$ measured over each site in a symmetric six dangling bond structure at different tip heights**. (**a**) Constant height $\Delta f$ image of the structure. (**b**, **c**)Histograms of the normalized $\Delta f$ measured over each dangling bond at (b) z = -320 pm and (c) z = -270 pm. 1600 line scans at both heights were used to gather statistics. Each histogram has 75 equal width bins between $\Delta f$(normalized) = 0 and 1.5, and has an integrated area of 1.0. All the dangling bonds appear negatively charged in (b). In (c), the isolated dangling bonds on either end (blue and yellow) remain negatively charged while the outer atoms of each pair (green and purple) are neutral. In (c) the inner atoms (red and cyan) fluctuate between the neutral and negative charge states; the integrated area of each peak is approximately 0.5, indicating they are equally likely to be in the neutral or negative charge state. This can be seen directly in Fig. 2d where a single electron switches between these two dangling bonds.

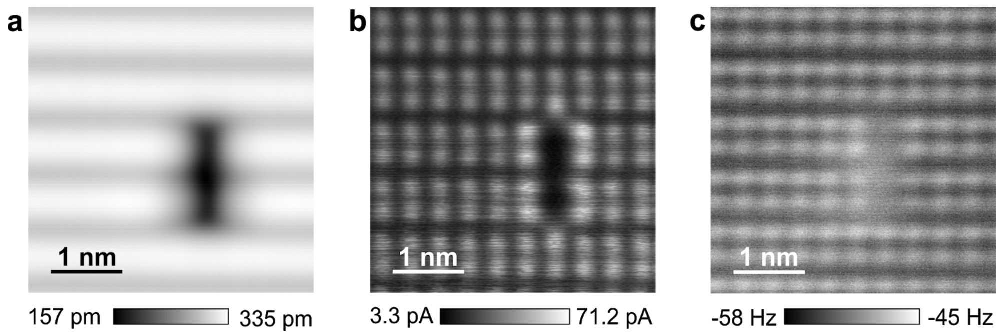


**Figure S4: Dimer vacancy in neighboring dimer rows on hydrogen-terminated Si(100).** (**a**) Constant current filled state STM image, -1.8V and 50 pA. (**b**) Constant height tunneling current image (300 mV, tip offset -370 pm). (**c**) Constant height $\Delta f$ image, 0V and tip offset -300 pm. Reference tip height for (b) and (c) is -1.8 V and 50 pA measured above hydrogen.

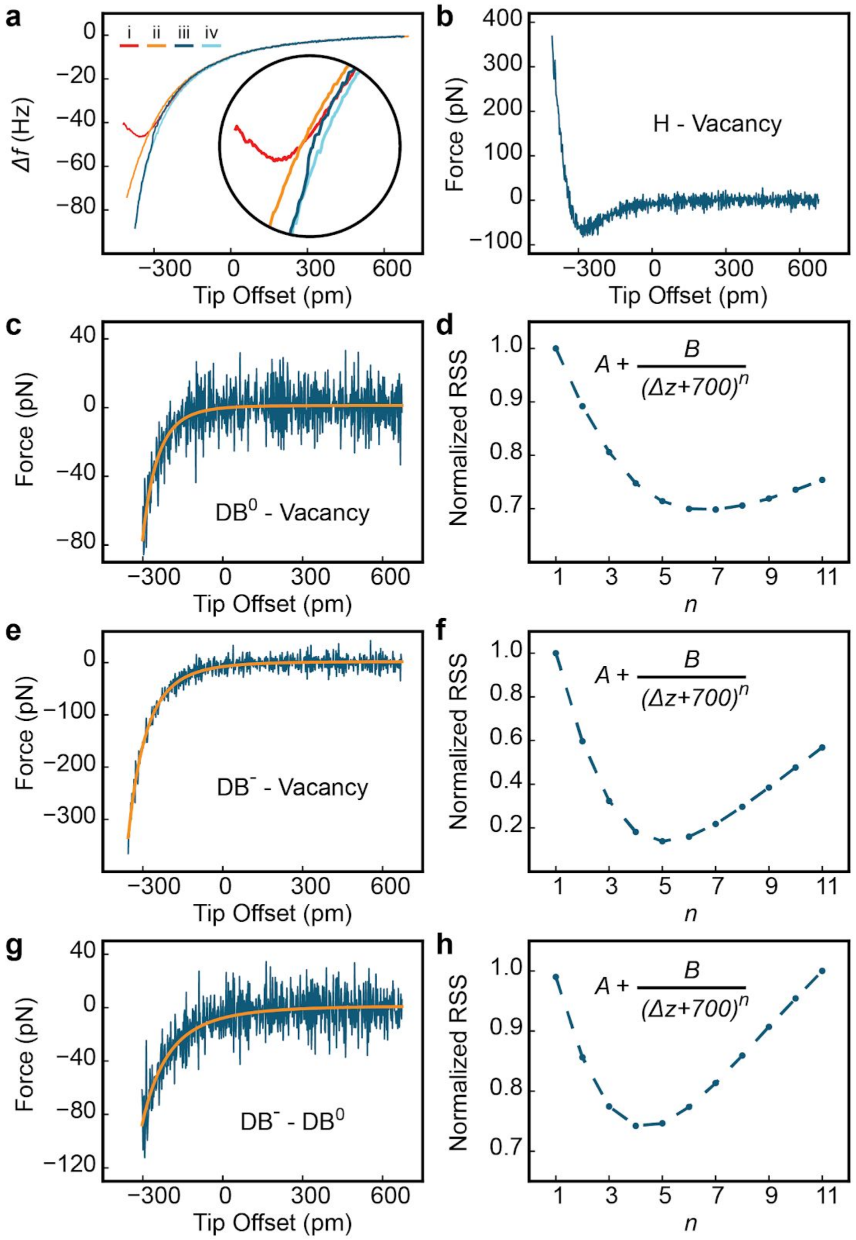


**Figure S5: Extraction of short range forces from Δ*f(z)* spectra.** **(a)** $\Delta f(z)$ taken over a hydrogen atom (i. red), dimer vacancy (ii. orange) and the right dangling bond of a pair (iii. dark blue, approach; iv. light blue, retract). $\Delta z$ = 0 corresponds to an STM setpoint of-1.8 V and 50 pA. All curves were taken at 0 V. Inset: a closeup of the spectra near $\Delta z$ = -300 pm. **(b)** The short range force measured over a hydrogen atom, corresponding to the difference in the force measured over the hydrogen atom and the dimer vacancy (forces found by converting $\Delta f(z)$ to force *via* Sader-Jarvis Method [4,5]. **(c, e, g)** The short range forces measured over a neutral and negatively charged dangling bond. The force for the neutral dangling bond corresponds to the approach curve in (a) (dark blue) up to the point of the sudden increase in $|\Delta f|$. The force for the negatively charged dangling bond corresponds to the retract curve in (a) (light blue). **(d, f, h)** Comparisons of the fits of the extracted short range forces for (c, e, g), respectively. RSS corresponds to the residual sum of squares error. The absolute tip height at the set point was determined to be 700 pm. Approaching the tip 700 pm from our setpoint typically results in sudden increases to the tunneling current and small changes to the tip apex and surface, strongly suggesting the tip makes direct contact with the hydrogen-free silicon surface.

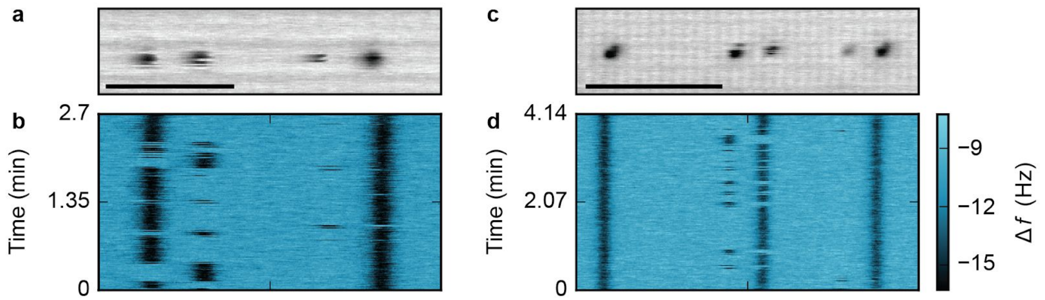


**Figure S6: The influence of adding an isolated dangling bond on the polarization of dangling bond pairs.** (**a**) Constant height $\Delta f$ image of a symmetric structure composed of four dangling bonds. (**b**) A line scan map composed of two hundred sequential $\Delta f$ line scans acquired over the structure demonstrate that it is naturally polarized. The negative charge confined to the left-hand pair favors the outer dangling bond but occasionally fluctuates to the inner dangling bond. The negative charge confined to the right-hand pair almost exclusively occupies the outer dangling bond. (**c**) An isolated dangling bond was added to the left of the *same* structure in (a) using STM lithography. (**d**) A line scan map composed of two hundred sequential $\Delta f$ line scans acquired over the structure demonstrate the effect of this additional negative charge to the polarization of the structure. The right-hand pair remains polarized in the same way as (b). The polarization of the left-hand pair reverses compared to (b). This is easily rationalized by noting that the new dangling bond acts as a local Coulombic bias. This demonstrates that local charges (*e.g.* negatively charged dangling bonds or ionized donors) can influence the distribution of charge configurations these structures display. The scale bars in (a) and (c) are 3 and 4 nm, respectively. The individual line scans acquired in (d) are longer than in (b) due to the increased distance the tip has to move. The $\Delta f$ colour bar applies to both (b) and (d).

## References

[1] T. R. Huff, H. Labidi, M. Rashidi, M. Koleini, R. Achal, M. H. Salomons, and R. A. Wolkow, ACS Nano **11**, 8636 (2017).

[2] S. R. Schofield, N. J. Curson, J. L. O'Brien, M. Y. Simmons, R. G. Clark, N. A. Marks, H. F. Wilson, G. W. Brown and M. E. Hawley, Phys. Rev. B **69**, 085312 (2004).

[3] N. J. Curson, S. R. Schofield, M. Y. Simmons, L. Oberbeck, J. L. O'Brien, and R. G. Clark, Phys. Rev. B **69**, 195303 (2004).

[4] J. E. Sader and S. P. Jarvis, Appl. Phys. Lett. **84**, 1801–1803 (2004).

[5] J. Welker, E. Illek and F. J. Giessibl, Beilstein J. Nanotechnol. **3**, 238–248 (2012).
